# Supplementary material for: Time-Constrained Learning
Source: arXiv:2202.01913 source file (2022-02-04)
Supplement: Supplementary file 1 [file 4_tct_dynamic.tex]

\subsection{A TCT with a dynamic $\alpha$ parameter}

We developed a version of the \TCT teacher with no fixed ratio between wrong and random examples provided to the learner at each round, i.e., with no $\alpha$ user input. Instead, this dynamic $\TCT$ sets $\alpha = 1-acc_1$ at each round\marginpar{\scriptsize  {\arabic{mynotes}.\ {\sf \textcolor{red}{P: Não sei se é de fato $\alpha = 1-acc_1$}}}}. Figure \ref{fig:tct-dynamic-vs-double-appendix} provides additional comparisons between the {\tt dynamic\_TCT}, {\tt Double} and \OSCT. The meaning of each point in the graphs is the same as the one in the Experiments section. The top left image compares {\tt dynamic TCT} with OSCT and the other five images present a comparison between {\tt dynamic TCT} and {\tt Double} for each of the Learners.

Figure \ref{fig:tct-dynamic-vs-double-appendix} indicates that {\tt dynamic\_TCT} is comparable to \TCT (with $\alpha=0.2$): both teachers outperform Double for all Learners but Decision Trees, where their performances are very similar. Moreover, {\tt dynamic\_TCT} has one less parameter than \TCT and does not face the issue of the set $A_2$ getting too big when $acc_1$ is big\footnote{Recall that \TCT builds a set $A_2$ with $\alpha|S| acc_1 / (1-acc_1)$ random exmples}.

\newcommand{\addAllDynvsDouble}{\includegraphics[width=19em]{appendix/TCT_dynamic_vs_Double/All learners - All datasets.png}}

\newcommand{\addDecTreeTCTDynvsDouble}{\includegraphics[width=19em]{appendix/TCT_dynamic_vs_Double/DecisionTree - All datasets.png}}

\newcommand{\addLGBMTCTDynvsDouble}{\includegraphics[width=19em]{appendix/TCT_dynamic_vs_Double/LGBM - All datasets.png}}

\newcommand{\addLogRegTCTDynvsDouble}{\includegraphics[width=19em]{appendix/TCT_dynamic_vs_Double/LogisticRegression - All datasets.png}}

\newcommand{\addRandForestTCTDynvsDouble}{\includegraphics[width=19em]{appendix/TCT_dynamic_vs_Double/RandomForest - All datasets.png}}

\newcommand{\addSVMLinTCTDynvsDouble}{\includegraphics[width=19em]{appendix/TCT_dynamic_vs_Double/SVMLinear - All datasets.png}}

\begin{figure}
\begin{center}
\begin{tabular}{l*2{C}@{}}
%\toprule
& \addAllDynvsDouble & \addDecTreeTCTDynvsDouble \\
& \addLogRegTCTDynvsDouble & \addSVMLinTCTDynvsDouble \\
& \addLGBMTCTDynvsDouble  &  \addRandForestTCTDynvsDouble  \\ 
%\bottomrule 
\end{tabular}
\end{center}
\caption{Average accuracies on testing set along normalized time for {\tt dynamic\_TCT}, {\tt Double} and \OSCT. The numbers next to the labels are their average accuracies at the last normalized time limit $t=1$. }
\label{fig:tct-dynamic-vs-double-appendix}
\end{figure}
