# Supplementary material for: Time-Constrained Learning
Source: arXiv:2202.01913 source file (2022-02-04)
Supplement: Supplementary file 2 [file 3_explicacao_de_como_rodar_o_metodo.tex]

\subsection{How to run our experiments}

%Uma explicação de como rodar o nosso método (link anonymous no bitbucket)
